# Supplementary material for: Texture-Preserving Diffusion Models for High-Fidelity Virtual Try-On
Source: arXiv:2404.01089 source file (2024-04-01)
Supplement: Supplementary file 1 [file X_suppl.tex]

\clearpage
\setcounter{page}{1}
\maketitlesupplementary
